# Supplementary material for: Low-Pass Filtering of Active Turbulent Flows to Liquid Substrates
Source: arXiv:2511.22701 ancillary file (2025-11-27)
Supplement: Supplementary file 1 [file SM.pdf]

# Supplemental Material for
# Low-Pass Filtering of Active Turbulent Flows to Liquid Substrates

Gianmarco Spera and Julia M. Yeomans
*Rudolf Peierls Centre for Theoretical Physics, University of Oxford, Oxford OX1 3PU, United Kingdom*

Sumesh P. Thampi
*Department of Chemical Engineering, Indian Institute of Technology, Madras, Chennai, India 600036 and Rudolf Peierls Centre for Theoretical Physics, University of Oxford, Oxford OX1 3PU, United Kingdom*
(Dated: November 27, 2025)

**Contents**

SI. Substrate transfer function 1
A. Velocity-velocity correlation function 2

SII. Viscoelastic substrates 2

SIII. Time-correlation functions 3

SIV. Misalignment between strain rates and stresses 4

SV. List of supplementary movies 7

References 7

The Supplemental Material (SM) contains details of the derivation of the theoretical and numerical results presented in the main text. In all the SM, Eq. (X) and Fig. X refer to equations and figures of the main text while Eq. (S.X) and Fig. SX refer to equations and figures that appear in the Supplemental Material. In Section SI, we detail the derivation of the substrate transfer function, Eq. (5), and then use the transfer function to describe the behaviour of the velocity-velocity correlation function in space. In Section SII, we consider viscoelastic substrates to show generalisation of our results to materials which are not purely viscous. In Section SIII, we show numerically how our results extend to time-correlation functions. In Section SIV, we make analytical progress on the misalignment between the strain-rate tensor in the substrate and the strain-rate tensor and the nematic tensor in the active layer. Finally, in Section SV we list and describe the supplementary movies.

## SI. Substrate transfer function

In this section, we detail the derivation of the substrate transfer function, Eq. (5) of the main text, and then discuss its relevance for determining the velocity-velocity correlation function in the substrate layer.

The starting point to derive Eq. (5) is the Navier-Stokes equation of the substrate, Eq. (3), which we report here for completeness,

$$\partial_k u^{\mathrm{s}}_k = 0 \ , \quad \rho^{\mathrm{s}} D_t u^{\mathrm{s}}_i = \partial_j \left(-P^{\mathrm{s}}\delta_{ij} + 2\eta^{\mathrm{s}} E^{\mathrm{s}}_{ij}\right) + \xi^{\mathrm{c}}(u^{\mathrm{a}}_i - u^{\mathrm{s}}_i) \ , \tag{S.1}$$

where $P^{\mathrm{s}}$ is the pressure, $\eta^{\mathrm{s}}$ is the substrate viscosity, and $E^{\mathrm{s}}_{ij}$ is the strain-rate tensor in the substrate fluid. In the limit of low Reynolds number, Eq. (S.1) reads:

$$0 = -\partial_i P^{\mathrm{s}} + \eta^{\mathrm{s}}\partial_{jj} u^{\mathrm{s}}_i + \xi^{\mathrm{c}}(u^{\mathrm{a}}_i - u^{\mathrm{s}}_i) \ , \tag{S.2}$$

where we used the fluid incompressibility to rewrite $2\partial_j E^{\mathrm{s}}_{ij} = \partial_j\left(\partial_i u^{\mathrm{s}}_j + \partial_j u^{\mathrm{s}}_i\right) = \partial_i\partial_j u^{\mathrm{s}}_j + \partial_{jj} u^{\mathrm{s}}_i = \partial_{jj} u^{\mathrm{s}}_i$ as $\partial_j u^{\mathrm{s}}_j = 0$. By Fourier transforming Eq. (S.2), we obtain

$$0 = iq_i \tilde{P}^{\mathrm{s}} - \eta^{\mathrm{s}} q^2 \tilde{u}^{\mathrm{s}}_i + \xi^{\mathrm{c}}(\tilde{u}^{\mathrm{a}}_i - \tilde{u}^{\mathrm{s}}_i) \ . \tag{S.3}$$

We then project out the pressure by multiplying Eq. (S.3) by $\mathcal{P}_{mi} = \left(\delta_{mi} - q_i q_m/q^2\right)$ to obtain

$$0 = -\eta^{\rm s} q^2 \tilde{u}^{\rm s}_m + \xi^{\rm c}(\tilde{u}^{\rm a}_m - \tilde{u}^{\rm s}_m) \ , \tag{S.4}$$

where we used fluid incompressibility in the two layers, *i.e.* $q_i \tilde{u}_i^{\rm s|a} = 0$, to write $\mathcal{P}_{mi}\tilde{u}_i^{\rm s|a} = \tilde{u}_m^{\rm s|a}$. Finally, by solving Eq. (S.4) for $\tilde{u}^{\rm s}_i$ we obtain

$$\tilde{u}^{\rm s}_m(q_j) = T(q)\tilde{u}^{\rm a}_m(q_j) \ , \quad T(q) \equiv \frac{1}{[1+(\tilde{\ell}^{\rm s})^2 q^2]} \ , \tag{S.5}$$

where $q = |q_j|$, and we introduced the substrate screening length scale $\tilde{\ell}^{\rm s} \equiv \sqrt{\eta^{\rm s}/\xi^{\rm c}}$. Equation (S.5) is Eq. (5) of the main text.

Equation (S.5) also allows us to relate the energy spectra $\mathcal{E}^{\rm s|a}(q) = \frac{1}{2}|\tilde{u}_i^{\rm s|a}|^2$ in the two layers via $\mathcal{E}^{\rm s}(q) = T^2(q)\mathcal{E}^{\rm a}(q)$, which is Eq. (6) of the main text. As shown in Fig. 3b, the ratio $R(q) \equiv \mathcal{E}^{\rm s}(q)/\mathcal{E}^{\rm a}(q)$ plateaus at small wave numbers but decays as $\sim 1/q^4$ for large wave numbers ($q > 2\pi/\tilde{\ell}^{\rm s}$), consistent with the predictions of Eq. (S.5). In Fig. S2a, we further show that the large wave-length decay is always recovered as $\xi^{\rm c}$ is varied by several orders of magnitude. Moreover, we note that the ratio $R(q)$ deviates from the theoretical prediction as $q^{\rm s} \propto \sqrt{\xi^{\rm c}}$ increases, see Fig. 3b. Indeed, as $q^{\rm s}$ increases, the term $q/q^{\rm s}$ becomes always more comparable with the neglected terms, and we thus deviate from the low-Reynolds number approximations. In Fig. S2b, we show that the theoretical prediction improves as the viscosity of the substrate $\eta^{\rm s}$ increases and hence the Reynolds number decreases.

Finally, we remark that the low-pass filtering effect of the substrate is robust upon varying the viscosity. In Fig. S2c, we plot the ratio $\ell^{\rm s}/\ell^{\rm a}$ as $\eta^{\rm s}$ is varied. $\ell^{\rm s}/\ell^{\rm a}$ increases in agreement with the intuition that the screening length $\tilde{\ell}^{\rm s} = \sqrt{\eta^{\rm s}/\xi^{\rm c}}$ controls the low-pass filtering of the substrate. Therefore, an increase in the viscosity $\eta^{\rm s}$ is *equivalent* to lowering the friction coupling $\xi^{\rm c}$.

### A. Velocity-velocity correlation function

Let us now show how we can make some analytical progress in deriving the velocity-velocity correlations in the substrate $C^{\rm s}_{vv}$. The latter can be expressed using the Fourier transform as

$$C^{\rm s}_{vv}(r) = \langle u^{\rm s}_k(\mathbf{r}_0+\mathbf{r})u^{\rm s}_k(\mathbf{r}_0)\rangle_{\mathbf{r}_0,t} = \mathcal{F}^{-1}\left(|\tilde{u}^{\rm s}_i|^2\right) \simeq \mathcal{F}^{-1}\left(\frac{|\tilde{u}^{\rm a}_i|^2}{[1+(\tilde{\ell}^{\rm s})^2q^2]^2}\right) = \mathcal{F}^{-1}\left(\frac{\mathcal{F}\left(C^{\rm a}_{vv}(r)\right)}{[1+(\tilde{\ell}^{\rm s})^2q^2]^2}\right) \ , \tag{S.6}$$

where $\mathcal{F}^{-1}$ denotes the inverse Fourier transform, and we used the approximated result of Eq. (S.5). We thus assume that the velocity-velocity correlations in the active layer $C^{\rm a}_{vv}(r)$ decay exponentially with a typical active length scale $\ell^a$. While this is a strong approximation for the correlation function, it still retains two main ingredients: a characteristic length scale and a monotonic decrease at small $r$. By substituting $C^{\rm a}_{vv}(r) = \exp(-r/\ell^a)$ into Eq. (S.6), we obtain

$$C^{\rm s}_{vv}(r) \simeq \mathcal{F}^{-1}\left\{\frac{\mathcal{F}\left(\mathrm{e}^{-r/\ell^a}\right)}{[1+(\tilde{\ell}^{\rm s})^2q^2]^2}\right\} = \frac{\ell^a e^{-\left(\frac{1}{\ell^a}+\frac{1}{\tilde{\ell}^{\rm s}}\right)x}\left[2(\ell^a)^3 e^{\frac{x}{\tilde{\ell}^{\rm s}}} + (\tilde{\ell}^{\rm s})^2 e^{\frac{x}{\ell^a}}(\tilde{\ell}^{\rm s}+x) - (\ell^a)^2 e^{\frac{x}{\ell^a}}(3\tilde{\ell}^{\rm s}+x)\right]}{2\left[(\ell^a)^2 - (\tilde{\ell}^{\rm s})^2\right]^2} \ . \tag{S.7}$$

Figure S1d shows Eq. (S.7) for different values of $\tilde{\ell}^{\rm s}$ at fixed $\ell^{\rm a} = 1$. Indeed, the resulting function decays over length scales that are larger than $\ell^{\rm a}$. As expected, the approximated $C^{\rm s}_{vv}$ approaches $C^{\rm a}_{vv}$ in the limit of $\tilde{\ell}^{\rm s} \to 0$. Although this argument is not quantitative, it serves to guide the intuition on the length scale transfer from the active layer to the substrate.

## SII. Viscoelastic substrates

In this section, we consider the case of non-Newtonian substrates and show how our results extend to other rheologies by modeling the substrate as a viscoelastic fluid. To do so, we start from the incompressible Navier-Stokes equation of the substrate S.1 and introduce an additional term in the substrate stress tensor $\Pi^{\rm s}_{ij}$

$$\Pi^{\rm s}_{ij} = P^{\rm s}\delta_{ij} + 2\eta^{\rm s} E^{\rm s}_{ij} + \sigma^{\rm ve}_{ij} \tag{S.8}$$

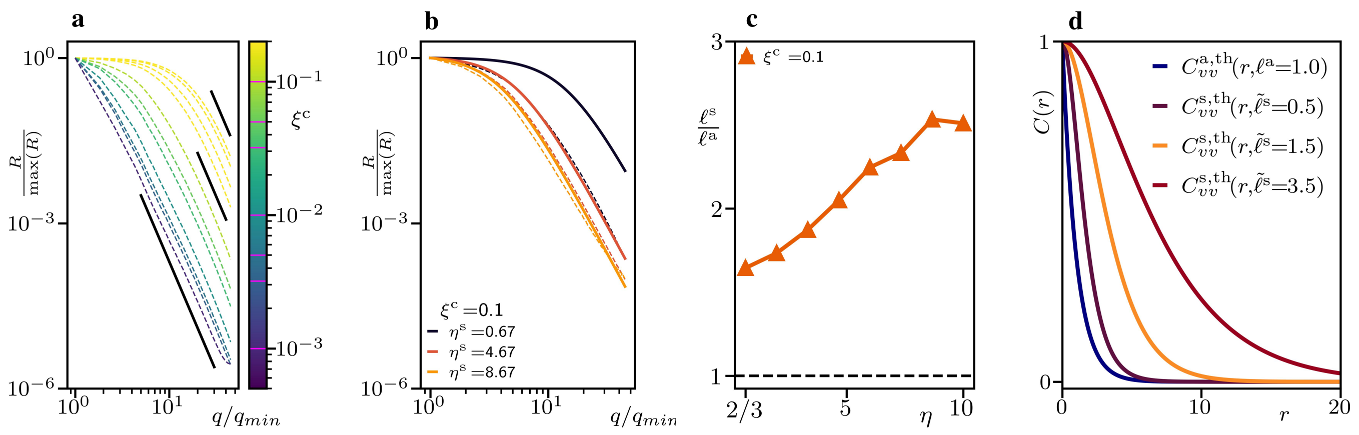


FIG. S1. **(a)** Spectral energy ratio $R \equiv \mathcal{E}^s(q)/\mathcal{E}^a(q)$ as the friction coupling is varied (for $\zeta = 0.01$). $R$ displays the predicted $R \sim 1/q^4$ (continuous black lines) behaviour for large q. As $\xi^c$ increases, such a scaling is recovered at larger wavelengths. Axes in (a) are normalized to make the comparisons clearer. **(b)** Spectral energy ratio $R \equiv \mathcal{E}^s(q)/\mathcal{E}^a(q)$ at fixed friction coupling $\xi^c = 0.1$ as the viscosity $\eta^s$ is varied. As $\eta^s$ increases, the Reynolds number decreases, and the theoretical prediction (continuous line) becomes more accurate compared to numerical measurements (dashed line). **(c)** Ratio $\ell^s/\ell^a$ at fixed $\xi^c = 0.1$ as the viscosity $\eta^s$ is varied. As $\eta^s$ increases, the length scale enlargement is still observed. **(d)** Velocity correlation in space computed using the simplified theory described by Eq. (S.7). As $\tilde{\ell}^s$ is varied, the resulting correlation $C^s_{vv}$ always decays over larger length scales than $\ell^a$ which is here kept fixed to one without loss of generality. Note that the decay length for $C^s_{vv}$ is larger than both $\ell^a$ and $\tilde{\ell}^s$.

where $\sigma^{ve}_{ij}$ is the viscoelastic stress tensor in the substrate fluid [? ]. In the following, we consider

$$\sigma^{ve}_{ij} = 2\eta^p E^s_{ij} + 2\varepsilon^{el} \int_0^t \mathrm{d}s E^s_{ij}(s) \qquad \text{(Kelvin-Voigt)} \qquad \text{(S.9a)}$$

$$\frac{\varepsilon^{el}}{\eta^s} \overset{\nabla}{\sigma^{ve}}_{ij} = -\sigma^{ve}_{ij} + 2\eta^p E^s \qquad \text{(Upper-convected Maxwell)} \qquad \text{(S.9b)}$$

where $\varepsilon^{el}$ is the substrate elasticity, $\eta^p$ is the polymeric viscosity, and $\overset{\nabla}{A}_{ij}$ is the upper-convected derivative of the tensor $A_{ij}$ defined as

$$\overset{\nabla}{A}_{ij} = \partial_t A_{ij} + u^s_k \partial_k A_{ij} + A_{ik}\partial_k u^s_j + \partial_i u^s_k A_{kj} \;, \qquad \text{(S.10)}$$

which ensures frame invariance. The case of a Kelvin-Voigt (Maxwell) substrate corresponds to a fluid composed of a spring and a dashpot connected in parallel (series). The substrate thus behaves as an elastic solid at long (short) time scales and as a viscous liquid at short (long) times. We solved Eqs. (1–3) of the main text with the substrate stress given by Eq. (S.8) at fixed substrate elasticity $\varepsilon^{el}$ as the friction coupling $\xi^c$ was varied. As shown in Fig. S2, the length-scale enlargement is still observed for both viscoelastic constitutive relations.

## SIII. Time-correlation functions

In this section, we study numerically the behaviour of time velocity-velocity correlations as friction coupling and the activity are varied. Velocity-velocity correlations in time in the active and substrate layers are defined as

$$C^a_{vv}(t) = \langle u^a_i(t_0) u^a_i(t_0+t)\rangle_{\mathbf{r},t_0} \quad \text{and} \quad C^s_{vv}(t) = \langle u^s_i(t_0) u^s_i(t_0+t)\rangle_{\mathbf{r},t_0} \;, \qquad \text{(S.11)}$$

where the average is performed over lattice sites $\mathbf{r}$ and initial time $t_0$, and plotted in Fig. S3a. Extracting characteristic time scales for the active and substrate layers, $\tau^a$ and $\tau^s$ respectively, we observe a similar behaviour as for the spatial length-scales reported in Fig. 2. The substrate enlarges time scales relative to the active layer, and the ratio $\tau^s/\tau^a$ slowly approaches unity in the limit of large $\xi^c$ (Figs. S3b,c).

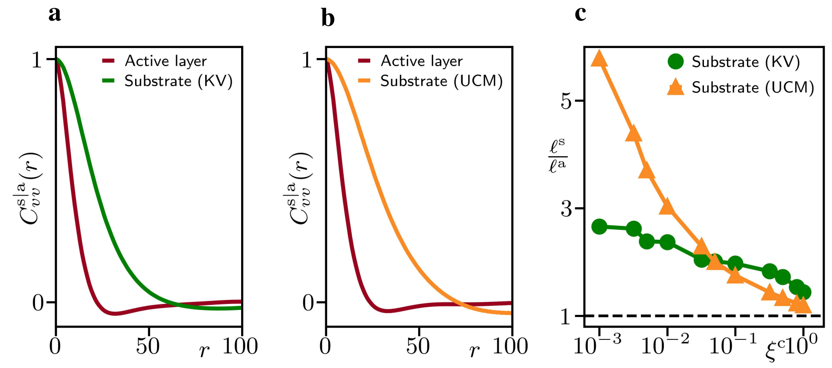


FIG. S2. Length-scale enlargement for Kelvin-Voigt (KV) and upper-convectd Maxwell (UCM) viscoelastic substrates (S.9). **(a-b)** Example of velocity-velocity correlations in space in the active layer and the substrate for the KV (a) and UCM (b). **(c)** Ratio $\ell^{\mathrm{s}}/\ell^{\mathrm{a}}$ as $\xi^{\mathrm{c}}$ is varied at fixed activity $\zeta = 0.01$ and elastic constant $\varepsilon^{\mathrm{el}} = 0.01$. $\ell^{\mathrm{s}}/\ell^{\mathrm{a}} > 1$ and, as the coupling coefficient increases, starts decreasing to unity. This curve quantifies how the low-pass filtering effect extends to viscoelastic substrates. Correlation lengths $\ell^{\mathrm{s|a}}$ are defined by the conditions $C_{vv}^{\mathrm{s|a}}(\ell^{\mathrm{s|a}}) = 1/e$. Simulation parameters are: $L_x = L_y = 400$, $\Gamma = 0.1$, $A = 0.1$, $K = 0.01$, $S_0 = 1$, $\lambda = 0.3$, $\eta^{\mathrm{a}} = \eta^{\mathrm{s}} = 2/3$, $\rho_0 = 20$, $\zeta = 0.01$, and $\eta^{\mathrm{p}} = 0$ for Kelvin-Voigt and $\eta^{\mathrm{p}} = 2/3$ for upper-convected Maxwell.

## SIV. Misalignment between strain rates and stresses

In this section, we derive the relations quantifying the misalignment between the strain-rate tensor in the substrate $E_{ij}^{\mathrm{s}}$ and the strain-rate tensor $E_{ij}^{\mathrm{a}}$ and the nematic tensor $Q_{ij}$ in the active layer.

To do so, we start by considering the Navier-Stokes equations for the two fluids, which we report here for complete-

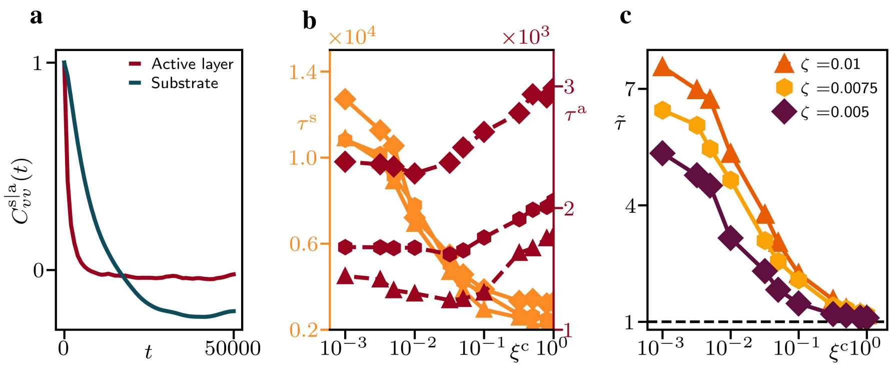


FIG. S3. **(a)** Examples of velocity-velocity correlation functions in time in the active layer (red) and in the substrate (blue), $C_{vv}^{\mathrm{a}}$ and $C_{vv}^{\mathrm{s}}$ respectively. $C_{vv}^{\mathrm{s}}$ decays over longer time scales than $C_{vv}^{\mathrm{a}}$. **(b)** Substrate and active time scales, $\tau^{\mathrm{s}}$ and $\tau^{\mathrm{a}}$ respectively, extracted from $C_{vv}^{\mathrm{s|a}}(t)$ as $\xi^{\mathrm{c}}$ is varied for three values of the activity $\zeta$. $\tau^{\mathrm{s}}$ is larger than $\tau^{\mathrm{a}}$ and decreases as $\xi^{\mathrm{c}}$ increases. $\tau^{\mathrm{a}}$ initially decreases as a result of substrate dissipation, and then increase again at large $\xi^{\mathrm{c}}$ as the substrate dissipation decreases, see also Fig. 2c. **(c)** Ratio $\tilde{\tau} \equiv \tau^{\mathrm{s}}/\tau^{\mathrm{a}}$ as $\xi^{\mathrm{c}}$ is varied. As friction increases, $\tilde{\tau}$ decreases to unity. Correlation times $\tau^{\mathrm{a}}$ and $\tau^{\mathrm{s}}$ are defined, respectively, by the conditions $C_{vv}^{\mathrm{a}}(\tau^{\mathrm{a}}) = 1/e$ and $C_{vv}^{\mathrm{s}}(\tau^{\mathrm{s}}) = 1/e$. Common simulation parameters are: $L_x = L_y = 400$, $\Gamma = 0.1$, $A = 0.1$, $K = 0.01$, $S_0 = 1$, $\lambda = 0.3$, $\eta^{\mathrm{a}} = \eta^{\mathrm{s}} = 2/3$, $\rho_0 = 20$. Panel (a) represents curves for $\zeta = 0.01$ and $\xi^{\mathrm{c}} = 0.01$.

ness:

$$\rho^{\mathrm{a}} D_t u_i^{\mathrm{a}} = \partial_j \Pi_{ij}^{\mathrm{a}} - \xi^{\mathrm{c}}(u_i^{\mathrm{a}} - u_i^{\mathrm{s}}) \ , \tag{S.12a}$$

$$\rho^{\mathrm{s}} D_t u_i^{\mathrm{s}} = \partial_j \Pi_{ij}^{\mathrm{s}} + \xi^{\mathrm{c}}(u_i^{\mathrm{a}} - u_i^{\mathrm{s}}) \ . \tag{S.12b}$$

We consider the limit of low Reynolds number, hence we neglect the left-hand-side in Eq. S.12. We then neglect the backflow contributions in Eq. S.12a and thus approximate $\Pi_{ij}^{\mathrm{pass}} \simeq -P^{\mathrm{a}}\delta_{ij}$. This is justified because the active driving generates stresses which dominate the backflow. Under these assumptions, Eq. (S.12) reduces to

$$0 = \partial_j \left[2\eta^{\mathrm{a}} \partial_j u_i^{\mathrm{a}} - P^{\mathrm{a}}\delta_{ij} - \zeta Q_{ij}\right] - \xi^{\mathrm{c}}(u_i^{\mathrm{a}} - u_i^{\mathrm{s}}) \ , \tag{S.13a}$$

$$0 = \partial_j \left[2\eta^{\mathrm{s}} \partial_j u_i^{\mathrm{s}} - P^{\mathrm{s}}\delta_{ij}\right] + \xi^{\mathrm{c}}(u_i^{\mathrm{a}} - u_i^{\mathrm{s}}) \ , \tag{S.13b}$$

where we used the incompressibility of the two fluids to rewrite the viscous contributions as $2\eta^{\mathrm{a|s}}\partial_j E_{ij}^{\mathrm{a|s}} = \eta^{\mathrm{a|s}}\partial_{jj} u_i^{\mathrm{a|s}}$.

Let us first derive the misalignment in Fourier space between the strain-rate tensors in the substrate and in the active layer. To do so, we use the results of Sec. SI, where we showed that Eq. (S.13b) allows to relate the velocity in the two layers in Fourier space via $\tilde{u}_i^{\mathrm{s}} = [1 + \tilde{\ell}^2 q^2]^{-1} \tilde{u}_i^{\mathrm{a}}$. It is then easy to show that, in Fourier space, the strain-rate tensors can be rewritten as

$$2\tilde{E}_{ij}^{\mathrm{s|a}} = -i\left(q_i \tilde{u}_j^{\mathrm{s|a}} + q_j \tilde{u}_i^{\mathrm{s|a}}\right) \ . \tag{S.14}$$

Therefore, using Eq. (S.5), we obtain

$$\tilde{E}_{ij}^{\mathrm{s}} = T(q)\tilde{E}_{ij}^{\mathrm{s}} \ . \tag{S.15}$$

Interestingly, Eq. (S.15) predicts that the two strain rates have parallel directors in Fourier space as they differ only by a numerical factor $T(q)$ which affects the magnitude but not the direction. The misalignment in real space is thus the result of the inverse Fourier transform. Note that, the perfect alignment in Fourier space is also a consequence of the approximations in Eq. (S.5), as we expect the contribution from the neglected material derivative to also introduce non-local couplings in Fourier space.

To derive an expression for the misalignment angle in real space, we start by deriving an expression for the angle between the main directors of the two tensors, and then use Eq. (S.15) to account for the observed behaviour. As both $E_{ij}^{\mathrm{a}}$ and $E_{ij}^{\mathrm{s}}$ are traceless and symmetric, the relative angle $\varphi = \varphi^{\mathrm{s}} - \varphi^{\mathrm{s}}$, with $\varphi^{\mathrm{s|a}}$ the orientation of the main directors of $E_{ij}^{\mathrm{s}}$ and $E_{ij}^{\mathrm{a}}$ respectively, is uniquely determined by the relation

$$\cos(2\varphi) = \cos(2\varphi^{\mathrm{a}})\cos(2\varphi^{\mathrm{s}}) + \sin(2\varphi^{\mathrm{a}})\sin(2\varphi^{\mathrm{s}}) = \frac{2(E_{xx}^{\mathrm{a}}E_{xx}^{\mathrm{s}} + E_{xy}^{\mathrm{a}}E_{xy}^{\mathrm{s}})}{|E_{sp}^{\mathrm{s}}||E_{qr}^{\mathrm{a}}|} = \frac{E_{ij}^{\mathrm{a}}E_{ij}^{\mathrm{s}}}{|E_{sp}^{\mathrm{s}}||E_{qr}^{\mathrm{a}}|} \tag{S.16}$$

where we introduced the norm $|E_{ij}^{\mathrm{s|a}}| \equiv \sqrt{E_{ij}^{\mathrm{s|a}}E_{ij}^{\mathrm{s|a}}}$. From Eq. (S.15) we can express $E_{ij}^{\mathrm{s}}$ as a function of $E_{ij}^{\mathrm{a}}$ in real space as

$$E_{ij}^{\mathrm{s}}(\mathbf{r}) = \frac{1}{2\pi(\tilde{\ell}^{\mathrm{s}})^2}(K_0 * E_{ij}^{\mathrm{a}})(\mathbf{r}) = \frac{1}{2\pi(\tilde{\ell}^{\mathrm{s}})^2}\int \mathrm{d}\mathbf{r}' \ K_0\left(\frac{|\mathbf{r}-\mathbf{r}'|}{\tilde{\ell}^{\mathrm{s}}}\right) E_{ij}^{\mathrm{a}}(\mathbf{r}') \ , \tag{S.17}$$

where $K_0$ is the modified Bessel function of the second kind, and we used that the Fourier transform of a convolution is the product of the Fourier transforms with

$$\mathcal{F}^{-1}\left[T(q)\right] = \int \frac{\mathrm{d}\mathbf{q}}{(2\pi)^2}\frac{\mathrm{e}^{-i\mathbf{q}\cdot\mathbf{r}}}{1 + (\tilde{\ell}^{\mathrm{s}})^2 q^2} = \int \frac{\mathrm{d}\mathbf{q}}{(2\pi)^2} T(q)\mathrm{e}^{-i\mathbf{q}\cdot\mathbf{r}} = \frac{1}{2\pi(\tilde{\ell}^{\mathrm{s}})^2} K_0\left(\frac{r}{\tilde{\ell}^{\mathrm{s}}}\right) \ . \tag{S.18}$$

Therefore, Eq. (S.16) can be rewritten as

$$\cos(2\varphi(\mathbf{r})) = \frac{\int \mathrm{d}\mathbf{r}' \ K_0\left(\frac{|\mathbf{r}-\mathbf{r}'|}{\tilde{\ell}^{\mathrm{s}}}\right) E_{ij}^{\mathrm{a}}(\mathbf{r}')E_{ij}^{\mathrm{a}}(\mathbf{r})}{|E_{sp}^{\mathrm{a}}(\mathbf{r})|\left|\int \mathrm{d}\mathbf{r}' \ K_0\left(\frac{|\mathbf{r}-\mathbf{r}'|}{\tilde{\ell}^{\mathrm{s}}}\right) E_{qr}^{\mathrm{a}}(\mathbf{r}')\right|} \ , \tag{S.19}$$

which is Eq. (8) of the main text.

We now show how Eq. (S.16) can be used to infer information about the average $\varphi$. We start by considering the spatial average of Eq. (S.16) which reads

$$\langle \cos(2\varphi(\mathbf{r}))\rangle_{\mathbf{r}} = \langle \frac{E^{\rm a}_{ij}E^{\rm s}_{ij}}{|E^{\rm s}_{sp}||E^{\rm a}_{qr}|}\rangle_{\mathbf{r}} = \frac{1}{\Omega}\int_{\Omega} {\rm d}\mathbf{r}\ \frac{E^{\rm a}_{ij}E^{\rm s}_{ij}}{|E^{\rm s}_{sp}||E^{\rm a}_{qr}|}\ , \tag{S.20}$$

where the space average is taken over the domain $\Omega$. Equation (S.20) cannot be easily manipulated, however, in the limit of fast-relaxing norms, we can simplify it as

$$\langle \cos(2\varphi(\mathbf{r}))\rangle_{\mathbf{r}} = \langle \frac{E^{\rm a}_{ij}E^{\rm s}_{ij}}{|E^{\rm s}_{sp}||E^{\rm a}_{qr}|}\rangle_{\mathbf{r}} \simeq \frac{\langle E^{\rm a}_{ij}E^{\rm s}_{ij}\rangle_{\mathbf{r}}}{\langle|E^{\rm s}_{sp}|\rangle_{\mathbf{r}}\langle|E^{\rm a}_{qr}|\rangle_{\mathbf{r}}}\ . \tag{S.21}$$

Equation. (S.21) can now be rewritten using the results in Fourier space as

$$\begin{aligned}\Omega\langle E^{\rm a}_{ij}E^{\rm s}_{ij}\rangle_{\mathbf{r}} &= \int {\rm d}\mathbf{r}\left[\int \frac{{\rm d}\mathbf{q}}{(2\pi)^2}\tilde{E}^{\rm s}_{ij}(\mathbf{q}){\rm e}^{-i\mathbf{q}\cdot\mathbf{r}}\right]\left[\int \frac{{\rm d}\mathbf{q}'}{(2\pi)^2}\tilde{E}^{\rm a}_{ij}(\mathbf{q}'){\rm e}^{-i\mathbf{q}'\cdot\mathbf{r}}\right] = \int \frac{{\rm d}\mathbf{q}\,{\rm d}\mathbf{q}'}{(2\pi)^4}\tilde{E}^{\rm s}_{ij}(\mathbf{q})\tilde{E}^{\rm a}_{ij}(\mathbf{q}')\int {\rm d}\mathbf{r}{\rm e}^{-i(\mathbf{q}+\mathbf{q}')\cdot\mathbf{r}} \\ &= \int \frac{{\rm d}\mathbf{q}}{(2\pi)^2}\ \tilde{E}^{\rm s}_{ij}(\mathbf{q})\tilde{E}^{\rm a}_{ij}(-\mathbf{q}) = \int \frac{{\rm d}\mathbf{q}}{(2\pi)^2}\ T(q)\tilde{E}^{\rm a}_{ij}(\mathbf{q})\tilde{E}^{\rm a}_{ij}(-\mathbf{q}) = \int \frac{{\rm d}\mathbf{q}}{(2\pi)^2}\ T(q)|\tilde{E}^{\rm a}_{ij}(\mathbf{q})|^2\ ,\end{aligned} \tag{S.22}$$

where we used that $E^{\rm a}_{ij}(-\mathbf{q}) = [E^{\rm a}_{ij}(\mathbf{q})]^*$. Since the integrand in Eq. (S.22) is always positive, the average $\langle\cos(2\varphi(\mathbf{r}))\rangle_{\mathbf{r}}$ in Eq. (S.21) is always positive. Therefore, the probability distribution $P(\varphi)$ of the relative angle $\varphi$ between $\{E^{\rm s}_{ij}, E^{\rm a}_{ij}\}$ is dominated by the values $\varphi < \pi/4$, in agreement with Fig. 4b of the main text.

Let us now consider the case of the relative angle $\chi$ between the strain-rate tensor in the substrate and the nematic tensor $Q_{ij}$. Following Eq. (S.20), the average of $\cos(2\chi)$ can be expressed as

$$\langle \cos(2\chi(\mathbf{r}))\rangle_{\mathbf{r}} = \langle \frac{E^{\rm s}_{ij}Q_{ij}}{|E^{\rm s}_{sp}||Q_{qr}|}\rangle_{\mathbf{r}} = \frac{1}{\Omega}\int_{\Omega} {\rm d}\mathbf{r}\ \frac{E^{\rm s}_{ij}Q_{ij}}{|E^{\rm s}_{sp}||Q_{qr}|}\ . \tag{S.23}$$

Using the fast norm approximation, and manipulating the numerator as in Eq. (S.22), we can rewrite $\langle E^{\rm s}_{ij}Q_{ij}\rangle_{\mathbf{r}}$ as

$$\langle E^{\rm s}_{ij}Q_{ij}\rangle_{\mathbf{r}} = \frac{1}{\Omega}\int {\rm d}\mathbf{r}\ E^{\rm s}_{ij}Q_{ij} = \frac{1}{\Omega}\int \frac{{\rm d}\mathbf{q}}{(2\pi)^2}\ E^{\rm s}_{ij}(\mathbf{q})Q_{ij}(-\mathbf{q})\ . \tag{S.24}$$

We thus need to find a relation between $E^{\rm s}_{ij}$ and $Q_{ij}$ in Fourier space as we did for $E^{\rm s}_{ij}$ and $E^{\rm a}_{ij}$.To do so, we differentiate Eq. (S.13a) to get

$$0 = 2\eta^{\rm a}\partial_k\partial_j\partial_j u^{\rm a}_i - \partial_k\partial_i P^{\rm a} - \partial_k\partial_j\zeta Q_{ij} - \xi^{\rm c}\partial_k(u^{\rm a}_i - u^{\rm s}_i)\ . \tag{S.25}$$

We then Fourier transform Eq. (S.13a) to obtain

$$0 = 2i\eta^{\rm a}q_k q^2[1+(\tilde{\ell}^{\rm s}q)^2]\tilde{u}^{\rm s}_i + q_k q_i P^{\rm a} + \zeta q_k q_j\tilde{Q}_{ij} + i\eta^{\rm s}q_k q^2\tilde{u}^{\rm s}_i\ , \tag{S.26}$$

where we used Eq. (S.5) to rewrite $\tilde{u}^{\rm a}_i = T^{-1}(q)\tilde{u}^{\rm s}_i = [1+(\tilde{\ell}^{\rm s}q)^2]\tilde{u}^{\rm s}_i$, and $(\tilde{\ell}^{\rm s})^2 = \eta^{\rm s}/\xi^{\rm c}$, to rewrite $\xi^{\rm c}(\tilde{u}^{\rm a}_i - \tilde{u}^{\rm s}_i) = \xi^{\rm c}\tilde{\ell}^2 q^2\tilde{u}^s_i = \eta^{\rm s}q^2\tilde{u}^s_i$. To lighten the notation, we recast Eq. (S.26) as

$$0 = iq_k G(q)\tilde{u}^{\rm s}_i + q_k q_i P^{\rm a} + \zeta q_k q_j\tilde{Q}_{ij}\ ,\quad G(q) \equiv [(\eta^{\rm a}+\eta^{\rm a})q^2 + \eta^{\rm a}\tilde{\ell}^2 q^4]\ . \tag{S.27}$$

We then project over the orthogonal components by multiplying Eq. (S.27) by $\mathcal{P}_{mi} = \left(\delta_{mi} - q_m q_i/q^2\right)$ to obtain

$$0 = iq_k G(q)\tilde{u}^{\rm s}_m + \zeta q_k q_j\tilde{Q}_{mj} - \zeta\frac{q_k q_m q_i q_j}{q^2}\tilde{Q}_{ij}\ , \tag{S.28}$$

where we used $\mathcal{P}_{mi}q_i P^{\rm a} = 0$ and fluid incompressibility $\mathcal{P}_{mi}\tilde{u}^{\rm s}_i = \tilde{u}^{\rm s}_m$.

To reconstruct the strain-rate tensor in the substrate, we add Eq. (S.28) to its transpose giving

$$0 = iG(q)(q_k\tilde{u}_m + q_m\tilde{u}_k) + \zeta\left(q_k q_j\tilde{Q}_{mj} + q_m q_j\tilde{Q}_{kj}\right) - 2\zeta\frac{q_k q_m q_i q_j}{q^2}\tilde{Q}_{ij}\ . \tag{S.29}$$

Substituting the expression for the strain-rate tensor of the substrate in Fourier space (S.14) into Eq. (S.29) gives

$$0 = G(q)\tilde{E}^{\rm s}_{km} - \zeta\left(q_k q_j\tilde{Q}_{mj} + q_m q_j\tilde{Q}_{kj}\right) + 2\zeta\frac{q_k q_m q_i q_j}{q^2}\tilde{Q}_{ij}\ . \tag{S.30}$$

Since $E^{\rm s}_{ij}$ and $Q_{ij}$ are symmetric and traceless, their Fourier transforms are also symmetric and traceless and we can decompose $\tilde{E}^{\rm s}_{ij}$ and $\tilde{Q}_{ij}$ as

$$\tilde{E}_{ij} = \tilde{\varepsilon}^{\rm s}\left(\gamma^{\rm s}_i\gamma^{\rm s}_j - \delta_{ij}/2\right) \quad \text{and} \quad \tilde{Q}_{ij} = \tilde{S}\left(n_i n_j - \delta_{ij}/2\right) \ . \tag{S.31}$$

Straightforward algebra then allows us to simplify Eq. (S.29) into

$$G(q)\tilde{\epsilon}^{\rm s}\left(\gamma^{\rm s}_k\gamma^{\rm s}_m - \frac{\delta_{km}}{2}\right) = \zeta\tilde{S}\left(q_k q_j n_m n_j + q_m q_j n_k n_j - 2\frac{q_k q_m q_i q_j}{q^2} n_i n_j\right) \ . \tag{S.32}$$

To derive an expression for the relative misalignment between $\tilde{E}_{ij}$ and $\tilde{Q}_{ij}$, we then contract Eq. (S.32) with $n_m n_k$ to obtain

$$G(q)\tilde{\epsilon}^{\rm s}\left[(\gamma^{\rm s}_i n_i)^2 - \frac{1}{2}\right] = \zeta\tilde{S}\left[2(n_i q_i)^2 - 2\frac{(n_i q_i)^4}{q^2}\right] \ , \tag{S.33}$$

where we have denoted $(n_i\gamma^{\rm s}_i)^2 = n_i\gamma^{\rm s}_i n_k\gamma^{\rm s}_k$ (and the same for higher order powers of contracted vectors). Eq. (S.33) can be solved for $(\gamma^{\rm s}_i n_i)^2$ to obtain

$$\cos^2(\tilde{\chi}) \equiv (n_i\gamma^{\rm s}_i)^2 = \frac{1}{2} + \frac{2\zeta\tilde{S}}{G(q)\tilde{\epsilon}^{\rm s}}(n_i q_i)^2\left[1 - \frac{(n_i q_i)^2}{q^2}\right] \ , \tag{S.34}$$

where we introduce $\tilde{\chi}$ as the angle between the director fields of the pair $\{\tilde{E}^{\rm s}_{ij}, \tilde{Q}_{ij}\}$ in Fourier space. Note that this angle is different from the corresponding angle in real space. Finally Eq. (S.34) can be rewritten as

$$\cos(2\tilde{\chi}) = \frac{4\zeta\tilde{S}}{G(q)\tilde{\epsilon}^{\rm s}}(n_i q_i)^2\left[1 - \frac{(n_i q_i)^2}{q^2}\right] = \zeta\frac{\tilde{S}}{\tilde{\epsilon}^{\rm s}}\frac{\mathcal{G}(q)}{2} \ , \quad \mathcal{G} \equiv \frac{8(n_i q_i)^2}{G(q)}\left[1 - \frac{(n_i q_i)^2}{q^2}\right] \tag{S.35}$$

where we introduced $\mathcal{G}$ to lighten the notation. Note that $\mathcal{G}$ is always positive. Using the result of Eq. (S.35) into Eq. (S.24), we obtain

$$\langle E^{\rm s}_{ij} Q_{ij}\rangle_{\mathbf{r}} = \frac{\zeta}{\Omega}\int\frac{{\rm d}\mathbf{q}}{(2\pi)^2}\,|\tilde{S}|^2\mathcal{G}(q) \ , \tag{S.36}$$

which implies that the sign of $\langle\cos(2\chi)\rangle$ in Eq. (S.23) is determined by the activity coefficient $\zeta$. As a result, the probability distribution $P(\chi)$ is dominated by $\chi < \pi/4$ for extensile activity ($\zeta > 0$) and by $\chi > \pi/4$ for contractile one ($\zeta < 0$). Interestingly, Eq. (S.36) also predicts a symmetric behaviour upon changing $\zeta \to -\zeta$, in agreement with the numerical measurements of $P(\chi)$ in Fig. 4d.

## SV. List of supplementary movies

In this section, we report all captions and parameters for the Supplementary Movies.

- **SM Movie 1.** Active turbulence and corresponding induced turbulence on the substrate. Simulation parameters are the same as in Fig. 1. Color represents the vorticity field $\omega^{\rm a|s} = (\partial_x u^{\rm a|s}_y - \partial_y u^{\rm a|s}_x)/2$. Blue (red) regions correspond to counterclockwise (clockwise) rotation.
- **SM Movie 2.** Coexistence of aligned and misaligned regions between pairs $\{E^{\rm s}_{ij}, E^{\rm a}_{ij}\}$ and $\{E^{\rm s}_{ij}, Q_{ij}\}$ for an extensile system. Simulation parameters are the same as in Fig. 4. Regions in which the tensorial quantities are aligned (angles between their directions between 0 and $\pi/4$) are coloured in blue whilst misaligned regions (angles between $\pi/4$ and $\pi/2$) are coloured in red.
- **SM Movie 3.** Coexistence of aligned and misaligned regions between pairs $\{E^{\rm s}_{ij}, E^{\rm a}_{ij}\}$ and $\{E^{\rm s}_{ij}, Q_{ij}\}$ for a contractile system. Simulation parameters are the same as in Fig. 4, but with an activity coefficient $\zeta = -0.01$. Regions in which the tensorial quantities are aligned are coloured in blue whilst misaligned regions are coloured in red. Note that for contractile activity, in contrast to extensile activity, regions of misalignment in $\{E^{\rm s}_{ij}, Q_{ij}\}$ dominate over aligned ones in agreement with Eq. (S.36).
